# Supplementary material for: Single-Spin Waved-Brim Flat-Top Hat in the Band Edge of GdIH Monolayer
Source: arXiv:2404.15007 source file (2024-04-23)
Supplement: Supplementary file 1 [file Supporing_Information-GdHI.pdf]

Supplemental Materials for

# Single-Spin Waved-Brim Flat-Top Hat in the Band Edge of GdIH Monolayer


Ningning Jia[1,*], Zhao Yang[1,*], Jiangtao Cai[2,*], Zhiheng Lv[1], Yongting Shi[1], Tielei Song[1], Xin Cui[1], Zhifeng Liu[1,†]

[1]*School of Physical Science and Technology, Inner Mongolia University, Hohhot 010021, China*

[2]*School of Physics and Information Science, Shaanxi University of Science and Technology, Xi' an 710021, China*


**TABLE OF CONTENTS**


**I. Dynamical and thermal stabilities of GdIH ML**

**II. Spin-polarized charge densities of different magnetic states**

**III. Curie temperature by the MFA method**

**IV. The fitted parameters for the WF-hat of GdIH ML**

**V. Electronic band structures of GdIH ML by different methods**

**VI. The method for the calculation of Berry curvature**

**VII. Anomalous valley Hall effect in GdIH ML**

**VIII. Carrier mobilities of unstrained and strained GdIH ML**

**IX. Orbital-resolved band structure of GdIH ML**

**X. The expression of the coefficients in Eqs.5-7**

**XI. The fitted on-site energies and hoping parameters**

**XII. Electronic band structures of GdIH ML under strains from −6%~6%**

**XIII. The band structure of −6%-strained GdIH ML with electron doping**


---


*These authors contributed equally to this work.

† Corresponding author: zfliu@imu.edu.cn

## I. Dynamical and thermal stabilities of GdIH ML

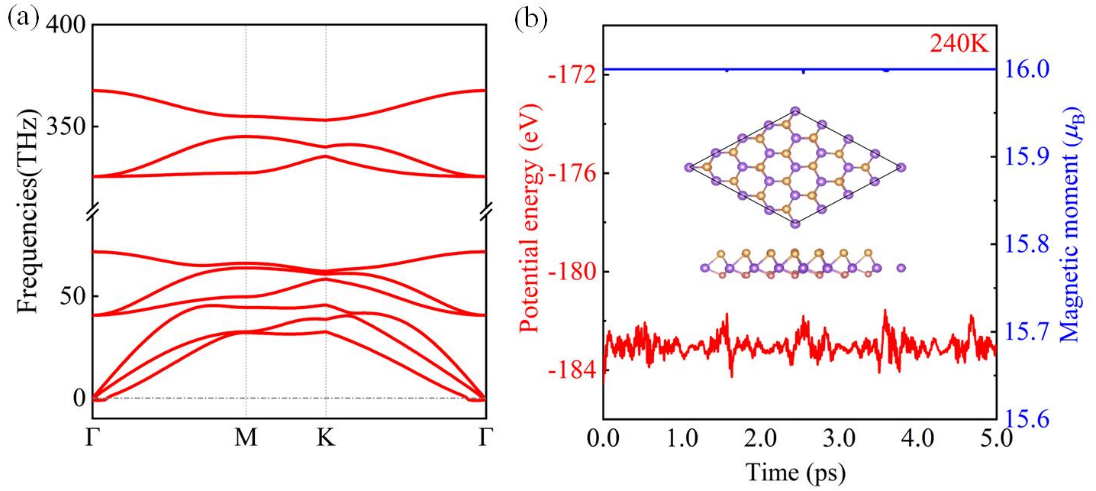


**FIG. S1.** (a) Phonon dispersion spectrum (b) Total potential energy fluctuation (red line) and the total magnetic moment (blue line) of (4 × 4 × 1) supercell for GdIH ML during first-principles molecular dynamic simulation at 240 K. The inset is the atomic structure at the end of the simulation time. Clearly, the structure does not collapse, indicating that it is thermally stable at the considered temperature.

## II. Spin-polarized charge densities of different magnetic states

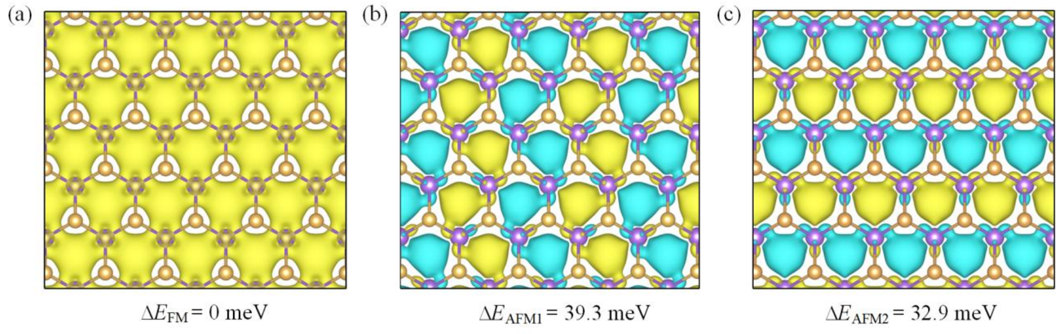


**FIG. S2.** The spatial distribution of spin-polarized charge density for GdIH ML in possible magnetic configurations: (a) FM, (b) AFM1 and (c) AFM2.

## III. Curie temperature by the MFA method

**Text S1:** Based on the obtained $J_1$ and $J_2$, the partition function Z of the system is expressed as

$$Z = \sum_{m=-M,-M+2,\ldots,M-2,M} \exp\left[\frac{(\gamma_1 J_1+\gamma_2 J_2)m<M>}{K_B T}\right], \quad \text{(SE1)}$$

here, $\gamma_1$ and $\gamma_2$ represent the first and second nearest-neighbor coordination numbers of the local moments, respectively. Since GdIH ML is a hexagonal lattice, one can establish the ensemble average of magnetic moment according to Eq. SE1:

$$<M> = \frac{1}{Z} \sum_{m=-M,-M+2,\ldots,M-2,M} m \times \exp\left[\frac{(\gamma_1 J_1 + \gamma_2 J_2)m<M>}{K_B T}\right]. \quad \text{(SE2)}$$

Here, we define

$$p = \frac{\gamma_1 J_1 + \gamma_2 J_2}{K_B T}. \quad \text{(SE3)}$$

Then, when the $M = 1$, the $<M>$ can be rewritten as

$$<M> = \frac{\mathrm{Sinh}(p<M>)}{\mathrm{Cosh}(p<M>)}. \quad \text{(SE4)}$$

So, it is easy to deduce that the critical point $p_c$ corresponds to the Curie temperature ($T_C$). As the value of $p_c$ is calculated to be 1 when $M = 1$, the MFA value of $T_C$ is estimated to be is 286 K.

## IV. The fitted parameters for the WF-hat of GdIH ML

**Table S1.** The fitted parameters (×$10^9$ eV Å) of $A_{j\text{-}i,i}$ parameters for the WF-hat of GdIH ML with *m*=7.

| ***j*** **= 0** | ***j*** **= 1** | ***j*** **= 2** | ***j*** **= 3** | ***j*** **= 4** | ***j*** **= 5** | ***j*** **= 6** | ***j*** **= 7** |
|---|---|---|---|---|---|---|---|
| $A_{0,0}$=1.38326 | $A_{1,0}$= 5.23076 | $A_{2,0}$=−11.74030 | $A_{3,0}$= 6.60518 | $A_{4,0}$=−1.59599 | $A_{5,0}$= 0.15605 | $A_{6,0}$= 0.00047 | $A_{7,0}$=−0.00067 |
| | $A_{0,1}$=−8.39540 | $A_{1,1}$= 1.22813 | $A_{2,1}$= 14.08310 | $A_{3,1}$=−9.01023 | $A_{4,1}$= 2.26433 | $A_{5,1}$=−0.24328 | $A_{6,1}$= 0.00814 |
| | | $A_{0,2}$= 13.83570 | $A_{1,2}$= −15.49840 | $A_{2,2}$= 0.29510 | $A_{3,2}$= 1.87447 | $A_{4,2}$=−0.49549 | $A_{5,2}$= 0.03818 |
| | | | $A_{0,3}$=−7.71771 | $A_{1,3}$= 9.73588 | $A_{2,3}$=−2.11897 | $A_{3,3}$= 0.04902 | $A_{4,3}$= 0.02213 |
| | | | | $A_{0,4}$= 1.94610 | $A_{1,4}$=−2.40764 | $A_{2,4}$= 0.50465 | $A_{3,4}$=−0.02956 |
| | | | | | $A_{0,5}$=−0.23982 | $A_{1,5}$= 0.27098 | $A_{2,5}$=−0.03553 |
| | | | | | | $A_{0,6}$= 0.01271 | $A_{1,6}$=−0.01182 |
| | | | | | | | $A_{0,7}$=−0.00008 |

## V. Electronic band structures of GdIH ML by different methods

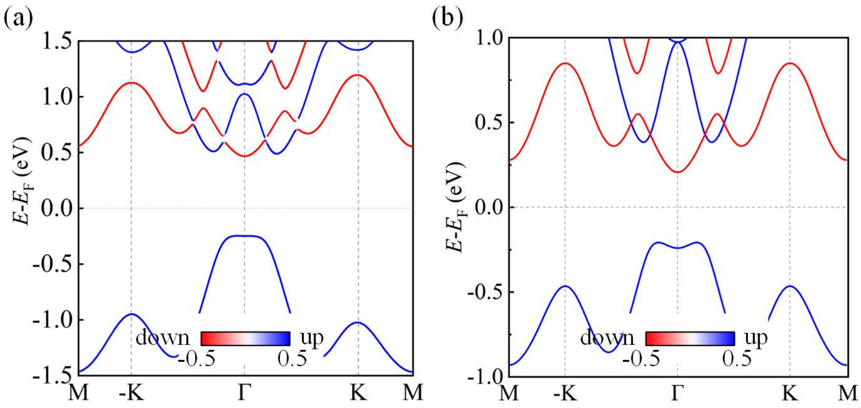


**FIG. S3.** Electronic band structures without SOC of GdIH ML from (a) HSE06 method
and (b) GGA+U method.

## VI. The method for the calculation of Berry curvature

**Text S2:** To characterize the valley-contrasting physics in GdIH ML, it is necessary to compute the Berry curvature according to the following expression. Under the Kubo formula, the *z*-component Berry curvature can be derived as

$$\Omega_z(\boldsymbol{k}) = \sum_n f_n \ \Omega_{n,z}(\boldsymbol{k}) \tag{SE5}$$

Here $f_n$ represents the Fermi-Dirac distribution, and $\Omega_{n,z}(\boldsymbol{k})$ can be obtained from

$$\Omega_{n,z}(\boldsymbol{k}) = -\sum_{n \neq n'} \frac{2\mathrm{Im}\langle \psi_{n\boldsymbol{k}} | v_x | \psi_{n'\boldsymbol{k}} \rangle \langle \psi_{n'\boldsymbol{k}} | v_y | \psi_{n\boldsymbol{k}} \rangle}{(E_n - E_{n'})^2} \ . \tag{SE6}$$

in which, $|\psi_{n\boldsymbol{k}}\rangle$ is the Bloch wave function with eigenvalue $E_n$, and $v_x$ ($v_y$) is the velocity operator along $x$ ($y$) direction.

## VII. Anomalous valley Hall effect in GdIH ML

As is known, the Berry curvature is an artificial gauge field, which can be considered as a pseudomagnetic field in the reciprocal space. Upon applying an in-plane electric field $E_{ext}$, the Bloch electrons in the valleys of ML GdIH will acquire an anomalous velocity to move towards transverse edge of GdIH ML, getting an anomalous velocity

$$v = \frac{1}{\hbar}\frac{\partial E_n(\boldsymbol{k})}{\partial \boldsymbol{k}} + \dot{\boldsymbol{k}} \times \Omega_z(\boldsymbol{k}) \tag{SE7}$$

For the conductive state under hole doping, the spin up holes at −K valley will be accumulated at the left edge of the sample, forming transverse Hall voltage (see Fig. S4a). Notably, if the magnetization is tuned from intrinsic $z$ direction to the $-z$ axis by external magnetic field, the spin down holes at K valley will move to opposite edges, and producing opposite Hall voltage (Fig. S4b).

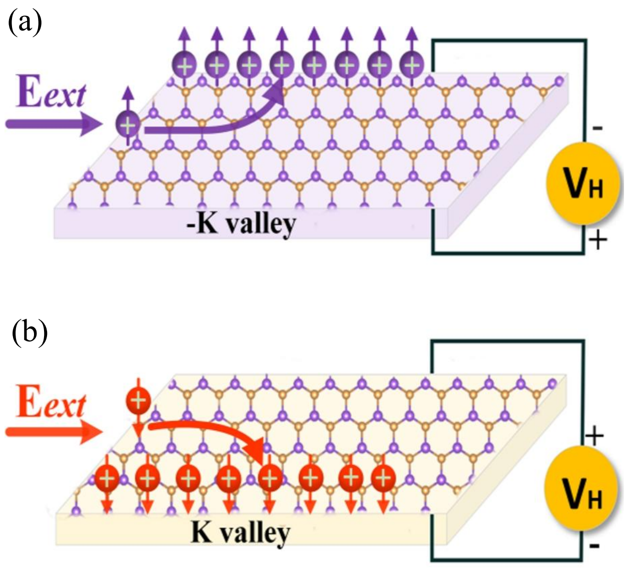


**FIG. S4.** Diagrams of the anomalous valley Hall effect under hole doping and an in-plane electric field with opposite magnetization: (a) $z$ direction (b) $-z$ direction.

**VIII. Carrier mobilities of GdIH ML**

**Text S3:** In the deformation potential theory, the carrier mobilities of 2D materials can be calculated by the expression:

$$\mu_{2D} = \frac{e\hbar^3 C_{2D}}{k_B T m_e^* m_d (E_l)^2}. \qquad \text{(SE5)}$$

Here, $m_e^*$ represents the effective mass in the transmission direction, $\hbar$ denotes the reduced Planck constant, and $k_B$ is the Boltzmann constant. $E_l$ refers to the deformation potential constant of the extremum of studied valleys, which is determined by $E_l = \Delta E/(\Delta l/l_0)$. Thereinto, $l_0$ is the lattice constant in the transmission direction, $\Delta l$ is the shape variable of $l_0$ stretching or compression (taken as −1.5%~1.5%), and $\Delta E$ is the change of the intrinsic energy of the extremum of valleys. $m_d$ denotes the average effective mass of carriers, defined as $m_d = \sqrt{m_x^* m_y^*}$. $C_{2D}$ is the elastic modulus of uniformly deformed lattice, which can be evaluated by the formula $C_{2D}$=2 $[\partial^2 E/\partial^2(\Delta l/l_0)]/S_0$, where $S_0$ is the optimized area and $E$ is the total energy of the system.

Based on the above methods, we calculate both of the electron (around the Γ valleys in the conductive band) and hole (around −K valley in the brim of WF-hat) mobilities for a redefined supercell of GdIH ML. The calculated $m^*$, $E_l$, $C_{2D}$ and the corresponding $\mu_{2D}$ are listed in Table S2. Moreover, we also present the fitted data for different $E_l$ and $C_{2D}$, see Fig. S5-S6.

**Table S2:** The obtained carrier mobilities of GdIH ML in the $x$ and $y$ directions around the −K valley in the WF-hat and Γ valley in conductive band. For comparison, we also calculated the carrier mobilities of black phosphorus (BP).

| **Systems** | **Effective mass** | | $E_{l\_x}$ | $E_{l\_y}$ | $C_{2D\_x}$ | $C_{2D\_x}$ | $\mu_{2D\_x}$ | $\mu_{2D\_y}$ |
|---|---|---|---|---|---|---|---|---|
| | $m_x^*/m_0$ | $m_y^*/m_0$ | (eV) | | (J/m$^2$) | | (10$^3$ cm$^2$V$^{-1}$s$^{-1}$) | |
| GdIH_*h* (−K) | 1.19 | 0.55 | 0.29 | 0.47 | 53.65 | 53.23 | 14 | 11 |
| GdIH_*e* ( Γ) | 0.76 | 0.48 | 1.90 | 1.69 | 53.65 | 53.23 | 0.7 | 1.4 |
| BP_*e* ( Γ) | 0.15 | 1.20 | | 5.43 | | 103.97 | | 0.14 |
| | 0.17[a] | 1.12[a] | | 7.11[a] | | 101.60[a] | | 0.08[a] |
| BP_*h* ( Γ) | 0.14 | 5.43 | | 0.87 | | 103.97 | | 24 |
| | 0.15[a] | 6.35[a] | | 0.15[a] | | 101.60[a] | | 10-26[a] |

[a]These data are cited from Ref [76] (i.e., *Nat. Commun*, 2014, 5, 4475)

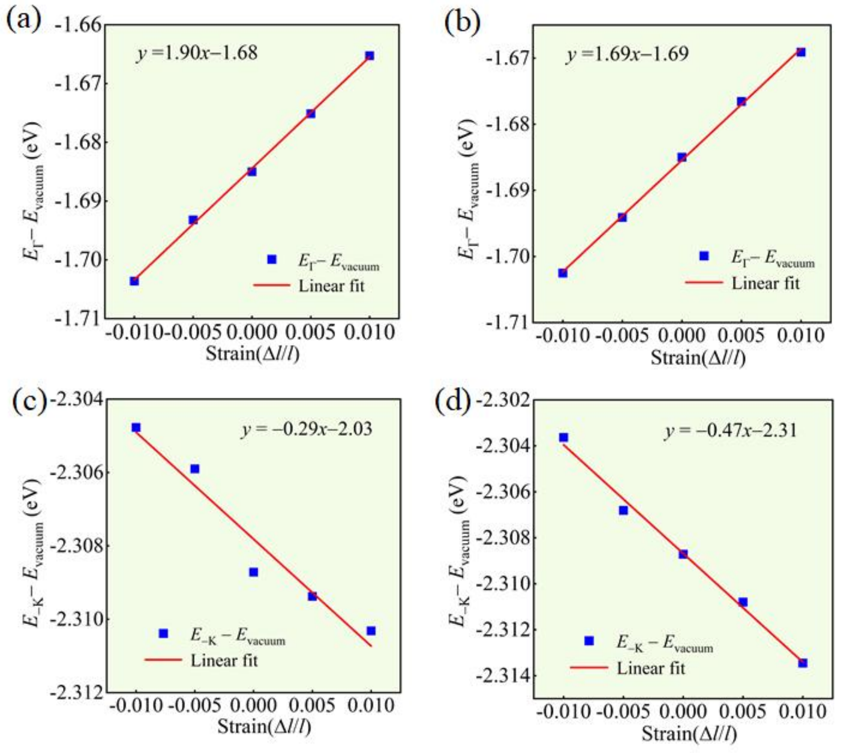


**FIG. S5.** The change of the energy at −K/Γ valley in valence/conductive band with respect to the applied uniaxial strain along (a/c) *x* or zigzag and (b/c) *y* or armchair directions.

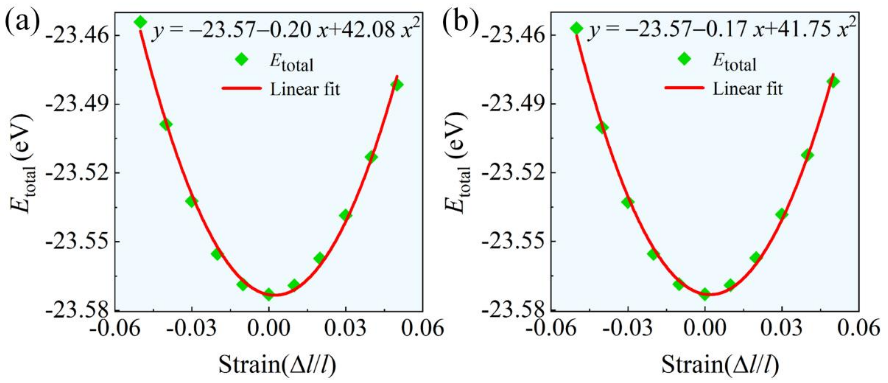


**FIG. S6.** The variation of total energy of GdIH ML with respect to the uniaxial strains along (a) *x* and (b) *y* directions. Based on the fitted second-order coefficients, the $C_{2D\_x}$ and $C_{2D\_y}$ are calculated to be 53.65 J/m$^2$ and 53.23 J/m$^2$, respectively.

## IX. Orbital-resolved band structure of GdIH ML

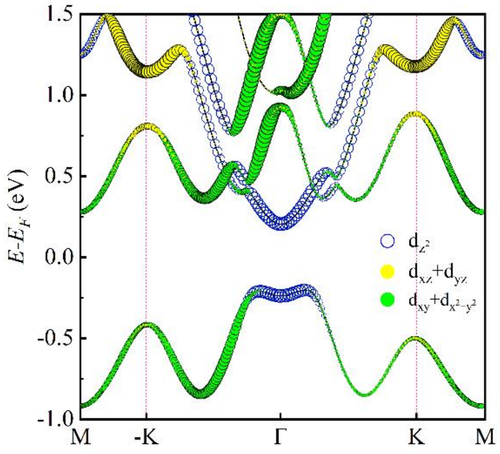


**FIG. S7.** Orbital-resolved band structure of GdIH ML with SOC from GGA+U method.

## X. The expression of the coefficients in Eqs.5-7

**Table S3. The relationships between the coefficients A$_{n,m}$, B$_{n,m}$, C$_{n,m}$, D$_{n,m}$, E$_{n,m}$, F$_{n,m}$ and different hoping parameters.**

| (*n*,*m*) | $A_{n,m}$ | $B_{n,m}$ | $C_{n,m}$ | $D_{n,m}$ | $E_{n,m}$ | $F_{n,m}$ |
|---|---|---|---|---|---|---|
| (0,1) | $-4\sqrt{3}\alpha_4 - 4\sqrt{3}\alpha_5 + 12\alpha_6$ | $4\sqrt{3}\alpha_1 + 4\sqrt{3}\alpha_2 - 12\alpha_3$ | $4\alpha_6$ | $-4\alpha_3$ | $6i\alpha_1 - 6i\alpha_2 - 6\alpha_4 - 6\alpha_5$ | $6\alpha_1 + 6\alpha_2 + 6i\alpha_4 - 6i\alpha_5$ |
| (0,2) | $-4\sqrt{3}\gamma_4 - 4\sqrt{3}\gamma_5 + 12\gamma_6$ | $4\sqrt{3}\gamma_1 + 4\sqrt{3}\gamma_2 - 12\gamma_3$ | $4\gamma_6$ | $-4\gamma_3$ | $6i\gamma_1 - 6i\gamma_2 - 6\gamma_4 - 6\gamma_5$ | $6\gamma_1 + 6\gamma_2 + 6i\gamma_4 - 6i\gamma_5$ |
| (1,0) | $2\sqrt{3}\alpha_4 + 2\sqrt{3}\alpha_5 + 16\alpha_6$ | $\frac{1}{6}(-2\sqrt{3}\alpha_1 - 2\sqrt{3}\alpha_2 - 12\alpha_3)$ | $-2\sqrt{3}\alpha_4 - 2\sqrt{3}\alpha_5 + 4\alpha_6$ | $\frac{1}{2}(2\sqrt{3}\alpha_1 + 2\sqrt{3}\alpha_2 - 4\alpha_3)$ | $\frac{1}{6}(6i\alpha_1 - 6i\alpha_2)$ | $6i\alpha_4 - 6i\alpha_5$ |
| (1,1) | $-4\sqrt{3}\alpha_4 - 4\sqrt{3}\alpha_5 + 12\alpha_6$ | $-4\sqrt{3}\alpha_1 - 4\sqrt{3}\alpha_2 - 12\alpha_3$ | $4\alpha_6$ | $4\alpha_3$ | $6i\alpha_1 - 6i\alpha_2 + 6\alpha_4 + 6\alpha_5$ | $6\alpha_1 + 6\alpha_2 - 6i\alpha_4 + 6i\alpha_5$ |
| (1, −1) | $8\sqrt{3}\beta_3 + 12\beta_4$ | $-12\beta_2$ | $4\beta_4$ | $4\beta_2$ | $-12i\beta_1 + 4i\sqrt{3}\beta_2 - 12\beta_3$ | $-4\sqrt{3}\beta_2$ |
| (1,2) | $-4\sqrt{3}\beta_3 + 12\beta_4$ | 0 | $4\sqrt{3}\beta_3 + 4\beta_4$ | 0 | $-12i\beta_1 + 4i\sqrt{3}\beta_2$ | $8\sqrt{3}\beta_2$ |
| (1,–2) | $3\delta_5 - 3\sqrt{3}\delta_6 - 3\sqrt{3}\delta_7 + 9\delta_8$ | $-3\delta_1 + 3\sqrt{3}\delta_2 + 3\sqrt{3}\delta_3 - 9\delta_4$ | $3\delta_5 + \sqrt{3}\delta_6 + \sqrt{3}\delta_7 + \delta_8$ | $-3\delta_1 - \sqrt{3}\delta_2 - \sqrt{3}\delta_3 - \delta_4$ | $6i\delta_2 - 6i\delta_3 - 3\sqrt{3}\delta_5 + 3\delta_6 + 3\delta_7 + 3\sqrt{3}\delta_8 + 6i\varepsilon_1$ | $3\sqrt{3}\delta_1 - 3\delta_2 - 3\delta_3 - 3\sqrt{3}\delta_4 + 6i\delta_6 - 6i\delta_7$ |

| | | | | | | |
|---|---|---|---|---|---|---|
| (1,3) | $3\delta_5 + 3\sqrt{3}\delta_6 + 3\sqrt{3}\delta_7 + 9\delta_8$ | $3\delta_1 + 3\sqrt{3}\delta_2 + 3\sqrt{3}\delta_3 + 9\delta_4$ | $3\delta_5 - \sqrt{3}\delta_6 - \sqrt{3}\delta_7 + \delta_8$ | $3\delta_1 - \sqrt{3}\delta_2 - \sqrt{3}\delta_3 + \delta_4$ | $6i\delta_2 - 6i\delta_3 - 3\sqrt{3}\delta_5 - 3\delta_6 - 3\delta_7 + 3\sqrt{3}\delta_8$ | $-3\sqrt{3}\delta_1 - 3\delta_2 - 3\delta_3 + 3\sqrt{3}\delta_4 - 6i\delta_6 + 6i\delta_7$ |
| (2,0) | $2\sqrt{3}\gamma_4 + 2\sqrt{3}\gamma_5 + 12\gamma_6$ | $-2\sqrt{3}\gamma_1 - 2\sqrt{3}\gamma_2 - 12\gamma_3$ | $-2\sqrt{3}\gamma_4 - 2\sqrt{3}\gamma_5 + 4\gamma_6$ | $2\sqrt{3}\gamma_1 + 2\sqrt{3}\gamma_2 - 4\gamma_3$ | $6i\gamma_1 - 6i\gamma_2$ | $6i\gamma_4 - 6i\gamma_5$ |
| (2,1) | $8\sqrt{3}\beta_3 + 12\beta_4$ | $-12\beta_2$ | $4\beta_4$ | $4\beta_2$ | $-12i\beta_1 + 4i\sqrt{3}\beta_2 + 12\beta_3$ | $4\sqrt{3}\beta_2$ |
| (2,–1) | $12\delta_5$ | $12\delta_1$ | $4\delta_8$ | $4\delta_4$ | $6i\delta_2 - 6i\delta_3 + 6\delta_6 + 6\delta_7$ | $6\delta_2 + 6\delta_3 - 6i\delta_6 + 6\delta_7$ |
| (2,2) | $-4\sqrt{3}\gamma_4 - 4\sqrt{3}\gamma_5 + 12\gamma_6$ | $-4\sqrt{3}\gamma_1 - 4\sqrt{3}\gamma_2 + 12\gamma_3$ | $4\gamma_6$ | $4\gamma_3$ | $6i\gamma_1 - 6i\gamma_2 + 6\gamma_4 + 6\gamma_5$ | $6\gamma_1 + 6\gamma_2 - 6i\gamma_4 + 6i\gamma_5$ |
| (2,3) | $3\delta_5 + 3\sqrt{3}\delta_6 + 3\sqrt{3}\delta_7 + 9\delta_8 + 6\varepsilon_2$ | $-3\delta_1 - 3\sqrt{3}\delta_2 - 3\sqrt{3}\delta_3 - 9\delta_4$ | $3\delta_5 - \sqrt{3}\delta_6 - \sqrt{3}\delta_7 + \delta_8$ | $-3\delta_1 + \sqrt{3}\delta_2 + \sqrt{3}\delta_3 - \delta_4$ | $6i\delta_2 - 6i\delta_3 + 3\sqrt{3}\delta_5 + 3\delta_6 + 3\delta_7 - 3\sqrt{3}\delta_8$ | $-3\sqrt{3}\delta_1 - 3\delta_2 - 3\delta_3 + 3\sqrt{3}\delta_4 + 6i\delta_6 - 6i\delta_7$ |
| (3,1) | $12\delta_5$ | $12\delta_1$ | $4\delta_8$ | $4\delta_4$ | $6i\delta_2 - 6i\delta_3 - 6\delta_6 - 6\delta_7$ | $-6\delta_2 - 6\delta_3 - 6i\delta_6 + 6\delta_7$ |
| (3,2) | $3\delta_5 - 3\sqrt{3}\delta_6 - 3\sqrt{3}\delta_7 + 9\delta_8$ | $-3\delta_1 + 3\sqrt{3}\delta_2 + 3\sqrt{3}\delta_3 - 9\delta_4$ | $3\delta_5 + \sqrt{3}\delta_6 + \sqrt{3}\delta_7 + \delta_8 + 2\varepsilon_2$ | $-3\delta_1 - \sqrt{3}\delta_2 - \sqrt{3}\delta_3 - \delta_4$ | $6i\delta_2 - 6i\delta_3 + 3\sqrt{3}\delta_5 - 3\delta_6 - 3\delta_7 - 3\sqrt{3}\delta_8$ | $-3\sqrt{3}\delta_1 + 3\delta_2 + 3\delta_3 + 3\sqrt{3}\delta_4 + 6i\delta_6 - 6i\delta_7$ |

**XI. The fitted on-site energies and hoping parameters.**

**Table S4. The fitted on-site energies and hoping parameters in the TB model Eq.3**

| On-site energies | nearest neighbor | next-neighbor | $3^{rd}$-neighbor | $4^{th}$-neighbor |
|---|---|---|---|---|
| $\varepsilon_1 = 0.0212$ | $\alpha_1 = 0.0118$ | $\beta_1 = 0.1187$ | $\gamma_1 = 0.0215$ | $\delta_1 = -0.0133$ |
| $\varepsilon_2 = -0.1388$ | $\alpha_2 = -0.0622$ | $\beta_2 = 0.0064$ | $\gamma_2 = -0.1105$ | $\delta_2 = -0.0001$ |
| | $\alpha_3 = -0.0132$ | $\beta_3 = 0.0933$ | $\gamma_3 = -0.0258$ | $\delta_3 = 0.0545$ |
| | $\alpha_4 = -0.0649$ | $\beta_4 = -0.0085$ | $\gamma_4 = -0.0238$ | $\delta_4 = 0.0153$ |
| | $\alpha_5 = 0.0269$ | | $\gamma_5 = -0.0094$ | $\delta_5 = -0.0041$ |
| | $\alpha_6 = 0.0499$ | | $\gamma_6 = -0.0269$ | $\delta_6 = 0.0033$ |
| | | | | $\delta_7 = -0.0299$ |
| | | | | $\delta_8 = -0.0268$ |

## XII. Electronic band structures of GdIH ML under strains from −6%~6%

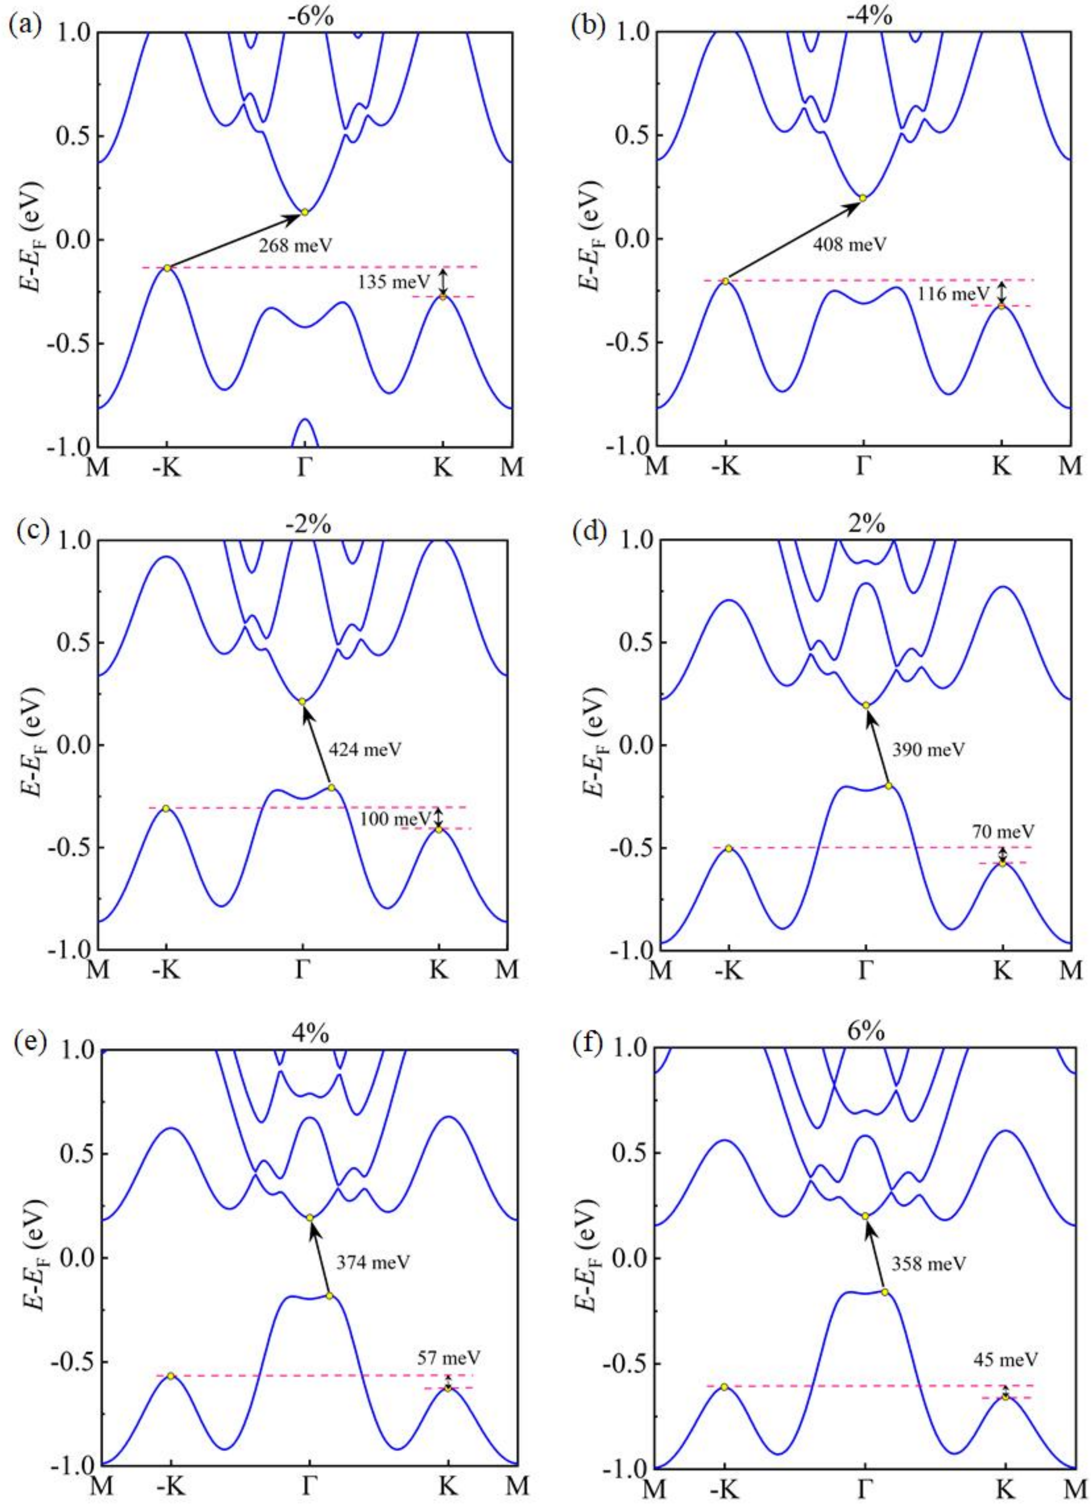


**Fig. S8** Electronic band structures of GdIH ML with SOC under strains from −6%~6%.

**XIII. The band structure of −6%-strained GdIH ML with electron doping**

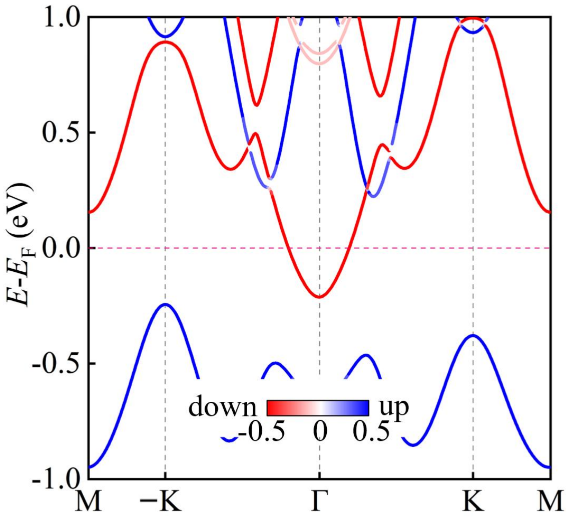


**FIG. S9.** The band structure of −6%-strained GdIH ML under carrier doping with a concentration of $7.97\times10^{13}$ cm$^{-2}$.
